# Supplementary material for: Revealing the formation and electrochemical properties of bis(trifluoromethanesulfonyl) imide intercalated graphite with first-principles calculations
Source: arXiv:1802.08775 source file (2018-02-24)
Supplement: Supplementary file 1 [file GIC-tfsi-supp.pdf]

# Supporting information – Revealing the formation and electrochemical properties of bis(trifluoromethanesulfonyl) imide intercalated graphite with first-principles calculations

Chol-Jun Yu,* Un-Song Ri, Gum-Chol Ri, and Jin-Song Kim

*Department of Computational Materials Design, Faculty of Materials Science, Kim Il Sung University, Ryongnam-Dong, Taesong District, Pyongyang, Democratic People's Republic of Korea*

Table S1. In-plane lattice constant ($a$), interlayer distance ($d_i$) and unit cell volume of graphie obtained with PBE, and PBE plus different vdW functionals.

| | $a$ (Å) | | $d_i$ (Å) | | Volume (Å$^3$) | |
|---|---|---|---|---|---|---|
| | Value | Error (%) | Value | Error (%) | Value | Error (%) |
| PBE | 2.4655 | 0.18 | 3.936 | 17.37 | 41.464 | 18.66 |
| vdW-DF | 2.4669 | 0.24 | 3.473 | 3.57 | 36.630 | 4.82 |
| vdW-DF2 | 2.4720 | 0.45 | 3.408 | 1.64 | 36.104 | 3.32 |
| vdW-DF-obk8 | 2.4630 | 0.08 | 3.259 | −2.82 | 34.262 | −1.95 |
| vdW-DF-ob86 | 2.4633 | 0.10 | 3.227 | −3.76 | 33.938 | −2.88 |
| vdW-DF2-b86r | 2.4635 | 0.10 | 3.225 | −3.83 | 33.917 | −2.94 |
| vdW-DF-cx | 2.4627 | 0.07 | 3.194 | −4.75 | 33.573 | −3.92 |
| vdW-DF2-c09 | 2.4628 | 0.07 | 3.181 | −5.13 | 33.441 | −4.30 |
| vdW-DF-c09 | 2.4623 | 0.05 | 3.153 | −5.98 | 33.128 | −5.30 |
| DFT-D | 2.4600 | −0.04 | 3.138 | −6.40 | 32.917 | −5.80 |
| Exp | 2.461 | | 3.353 | | 34.944 | |

Table S2. Löwdin charges of atoms in graphite, isolated TFSI molecule, and TFSI-$C_n$ compounds. Here, graphene means the graphene layer, and $C_{face}$ the carbon atoms facing the O and N atoms of TFSI, where the number in bracket indicates the number of $C_{face}$ atoms.

| | Graphite | TFSI | TFSI-$C_n$ | | | | |
|---|---|---|---|---|---|---|---|
| | | | 18 | 24 | 32 | 40 | 50 |
| Graphene | 3.962 | | 3.902 | 3.915 | 3.925 | 3.931 | 3.936 |
| $C_{face}$ | | | 3.894 (6) | 3.895 (3) | 3.898 (3) | 3.898 (1) | 3.900 (1) |
| TFSI | | 5.973 | 6.037 | 6.036 | 6.036 | 6.036 | 6.036 |
| N | | 5.751 | 6.009 | 5.982 | 5.964 | 5.955 | 5.945 |
| S | | 3.907 | 3.820 | 3.808 | 3.802 | 3.800 | 3.797 |
| C | | 3.245 | 3.347 | 3.347 | 3.351 | 3.354 | 3.359 |
| O | | 6.666 | 6.739 | 6.729 | 6.724 | 6.721 | 6.718 |
| F | | 7.147 | 7.209 | 7.221 | 7.228 | 7.231 | 7.235 |

*Corresponding author: Chol-Jun Yu, Email: ryongnam14@yahoo.com

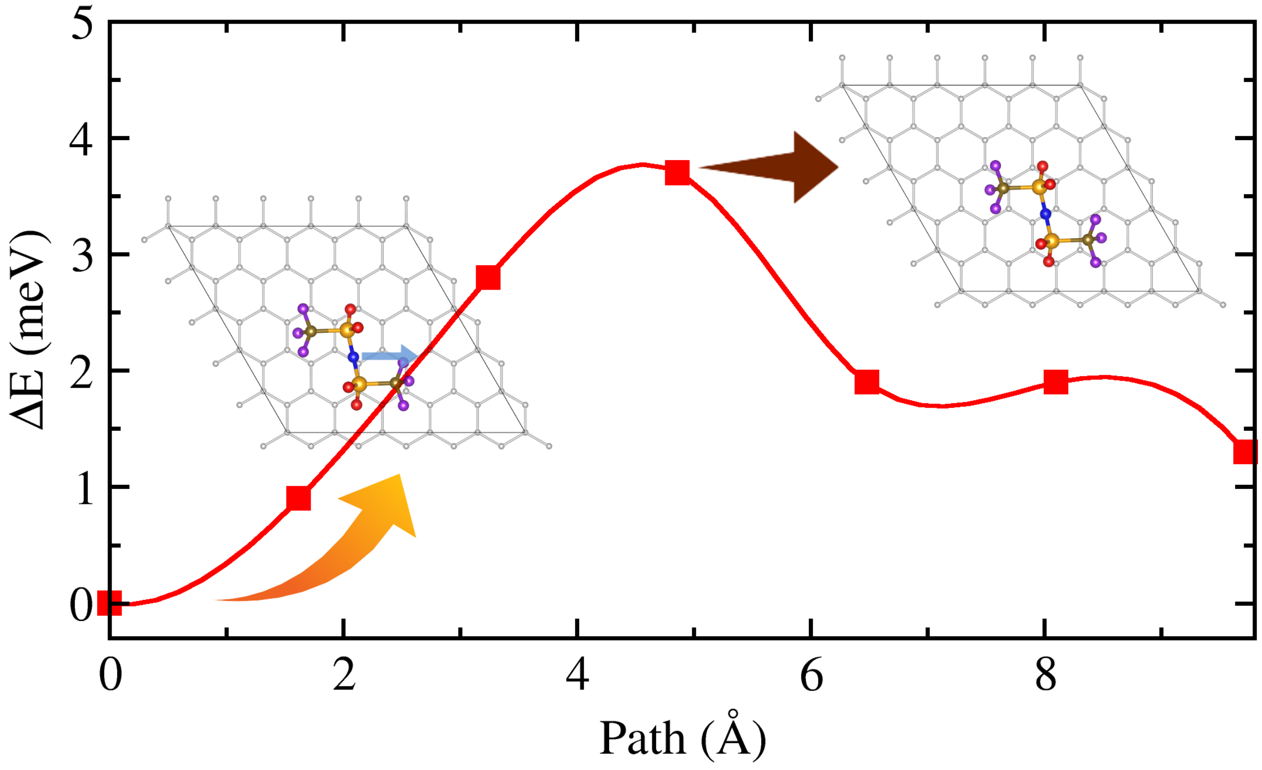


Figure S1. Activation barrier for TFSI migration along the path indicated by blue arrow, with the starting and transition states.

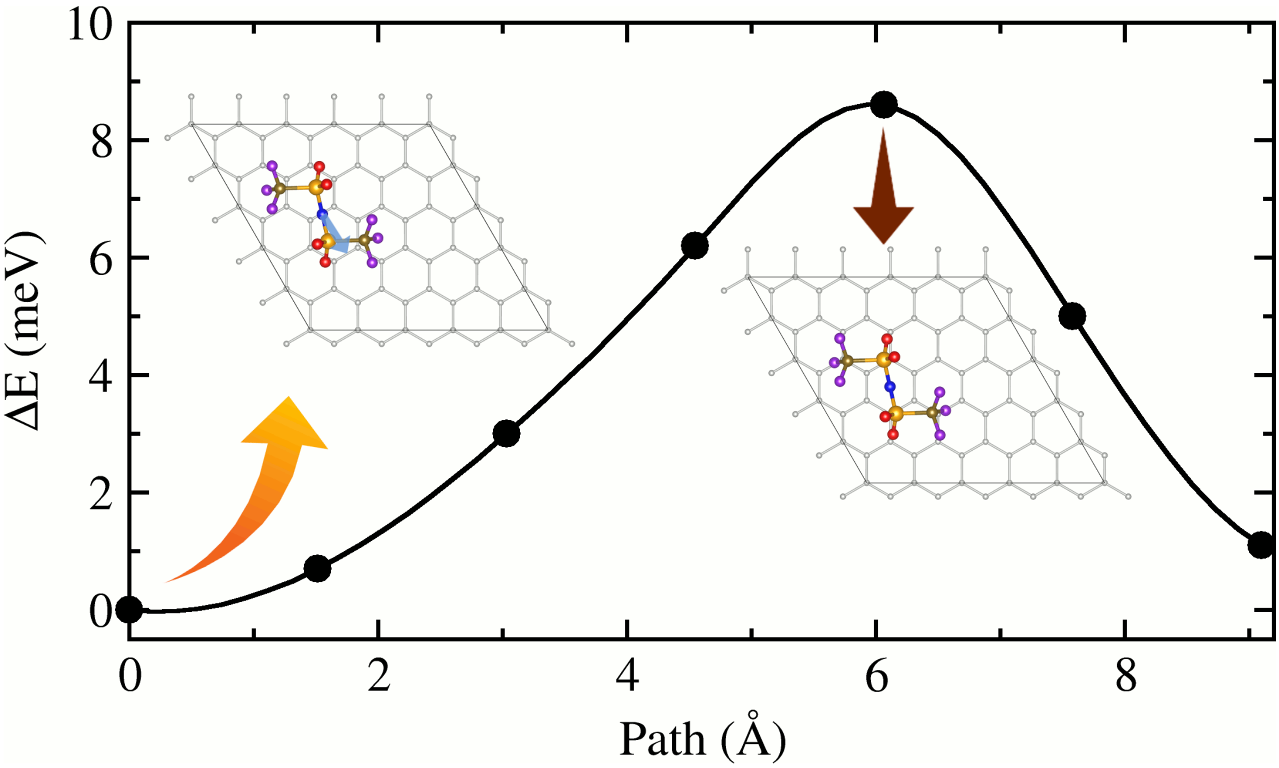


Figure S2. Activation barrier for TFSI migration along the path indicated by blue arrow, with the starting and transition states.

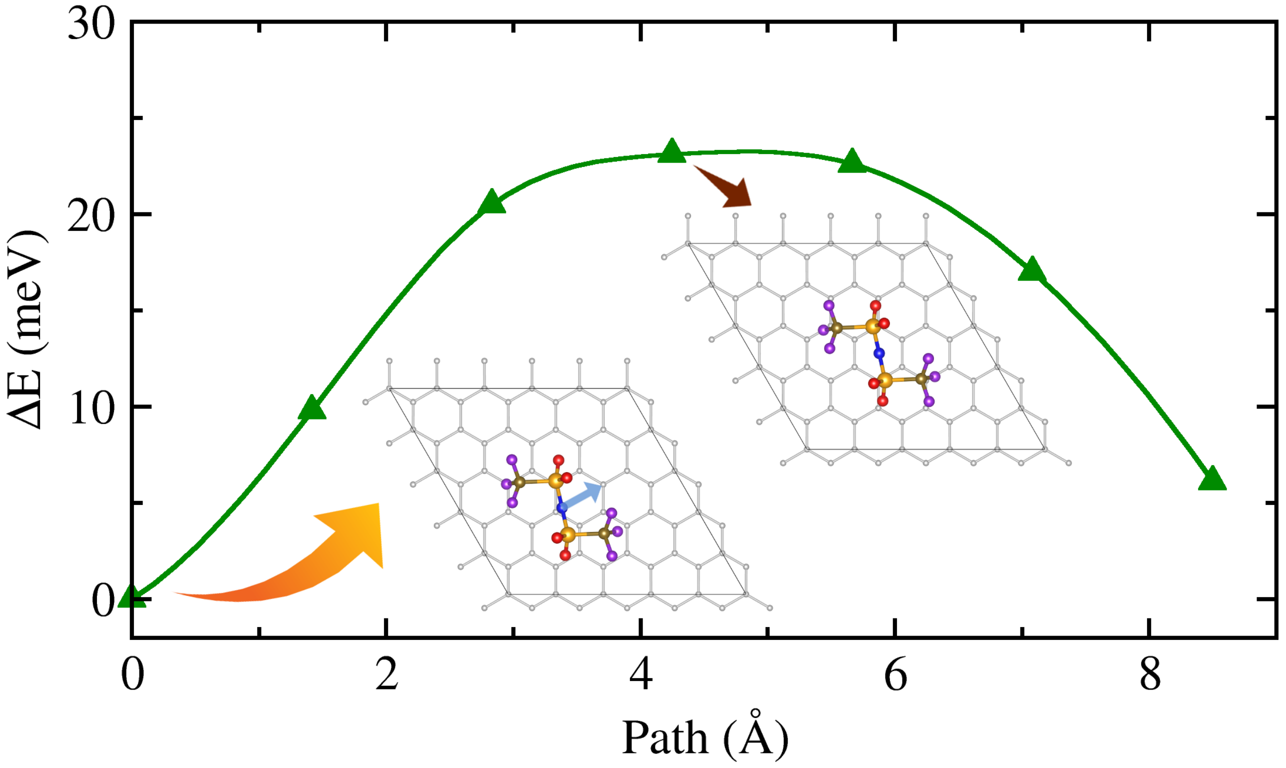


Figure S3. Activation barrier for TFSI migration along the path indicated by blue arrow, with the starting and transition states.
